# Supplementary material for: Mesoscale Organization and Dynamics in Binary Ionic Liquid Mixtures
Source: arXiv:1905.02827 ancillary file (2019-05-07)
Supplement: Supplementary file 1 [file supplementary_info.pdf]

## MATERIALS AND METHODS

### Experimental Details

1-octyl-3-methylimidazolium tetrafluoroborate ($C_8MIm\ BF_4$) and 1-ethyl-3-methylimidazolium tetrafluoroborate ($C_2MIm\ BF_4$) were purchased from Iolitec and dried under vacuum ($10^{-6}$ bar) at 60 °C for 24 hours prior to use. Broadband dielectric spectroscopy measurements were made in the frequency range of $10^{-1} - 10^{7}$ Hz using a Novocontrol Alpha Analyzer with a QUATRO liquid nitrogen temperature control system with temperature stability ±0.1 K. Samples were measured in a parallel plate capacitor geometry with 20 mm diameter gold-plated brass electrodes. A sample thickness of 1.6 mm was maintained using a Teflon spacer. The dynamic-mechanical spectra of the mixtures were obtained via oscillatory shear measurements over the frequency range 0.1 - 100 Hz and temperature range 220 - 190 K with 0.05 - 2 strain % on a Hybrid Rheometer 2 (TA Instruments) using parallel plate geometry with a diameter of 8 mm. The temperature was controlled by an Environmental Test Chamber with nitrogen as the gas source with temperature stability ±0.1K. Small-angle and wide-angle x-ray scattering measurements were conducted at room temperature using a SAXSLab Ganesha x-ray scattering system. The samples were encased in a button cell with Kapton windows. An empty cell was also measured to enable subtraction of the Kapton background. Differential scanning calorimetry measurements were performed on a TA Instruments Q2000 calorimeter at a cooling rate of 10 K/ min. The calorimetric glass transition temperature, $T_g$, was determined at the midpoint of the step in the heat flow corresponding to the maximum in the temperature derivative of the heat flow on cooling.

### Simulation Details

Molecular dynamics (MD) simulations for binary ionic liquid mixtures of $C_8MIm\ BF_4$ and $C_2MIm\ BF_4$ were carried out at a temperature of 298 K and pressure of 1 bar using GROMACS 2018 package, [1, 2] where $C_8MIm^+$ and $C_2MIm^+$ cations and $BF_4{}^-$ anion were modeled using a classical all-atom force field model developed by Canongia Lopes-Pádua [3, 4] (CL&P). Simulations for a total of three molar ratios (30:70, 50:50, and 70:30) obtained by varying the concentrations of the respective cations along with pure ionic liquid systems were performed. Simulations were conducted in a cubic box containing 2000 ion pairs with

periodic boundary conditions enforced in three dimensions. The temperature was controlled using Nosé-Hoover thermostat with a coupling constant of 0.4 ps while the pressure was maintained with Parrinello-Rahman barostat for which the coupling time constant was set to 2.0 ps. Appropriate tail corrections were applied for the non-bonded Lennard-Jones interactions while electrostatic interactions were handled using Particle Mesh Ewald (PME) method, each with a potential cutoff of 16 Å. The simulations were performed with a time step of 1 fs; coordinates were saved every 1 ps.

Each simulation was performed in four stages. First, low density initial configurations were generated using PACKMOL [5]. These initial configurations were then subjected to steepest descent minimization to remove high energy contacts followed by a 2 ns annealing scheme, where the temperature of the system was iteratively raised from 298 K to 498 K linearly in 200 ps followed by canonical ($NVT$) ensemble equilibration at 498 K for 100 ps and then brought down linearly to the desired temperature of 298 K in the next 200 ps. Additional relaxation of the system was achieved by simulating the systems in the $NVT$ ensemble for 10 ns, followed by a isothermal-isobaric ($NPT$) equilibration run of 20 ns. This cycle was repeated two more times. In the final cycle, the system was subjected to a 10 ns annealing scheme followed by $NVT$ and $NPT$ ensemble equilibration runs of 20 ns and 0.5 $\mu$s, respectively. After this, 0.5 $\mu$s of $NPT$ ensemble production run was conducted. The trajectories obtained from the final 40 ns were used for the structural analysis.

Structural properties of the ionic liquid systems are described in terms of x-ray structure factors and Voronoi domain analysis which were computed from MD simulation trajectories using tools implemented in TRAVIS. [6, 7] Further, the configuration snapshot visualization was rendered using VMD.[8]

## DIFFERENTIAL SCANNING CALORIMETRY

The DSC curves measured on cooling at 10 K/min are shown in Figure S1. The recorded calorimetric glass transition temperature, $T_g$, corresponds to the temperature at the peak in the derivative of heat flow with respect to time, inset Figure S1. The composition dependence of $T_g$, presented in Figure S2, follows the Fox equation for the glass transition in amorphous polymer blends, $1/T_g = (x_1/T_{g,1}) + (x_2/T_{g,2})$, where x is the mole fraction of each component IL, ant $T_{g,1}$ and $T_{g,2}$ are the transition temperatures of the neat ILs.[9] The $T_g$'s of the binary

IL mixtures are thus a weighted average of the two IL component $T_g$'s. The composition-dependent dielectric $\alpha$-relaxation rates, $\omega_{\alpha,BDS}$, and mechanical structural relaxation rates, $\omega_{\alpha,DMS}$, scale when plotted versus temperature normalized by $T_g$, see Figure S8. This indicates that these relaxations reflect the same dynamics which underlie the glass transition.

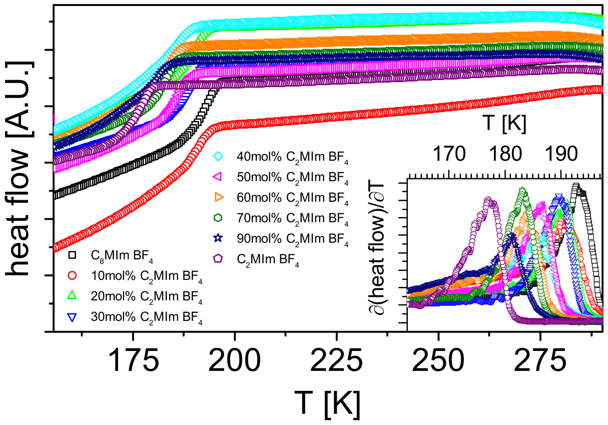


FIG. S1. Heat flow on cooling *versus* temperature as measured by differential scanning calorimetry. Inset: Derivative of heat flow with respect to temperature *versus* temperature. The calorimetric glass transition temperatures were recorded at the peak maximum of the derivative.

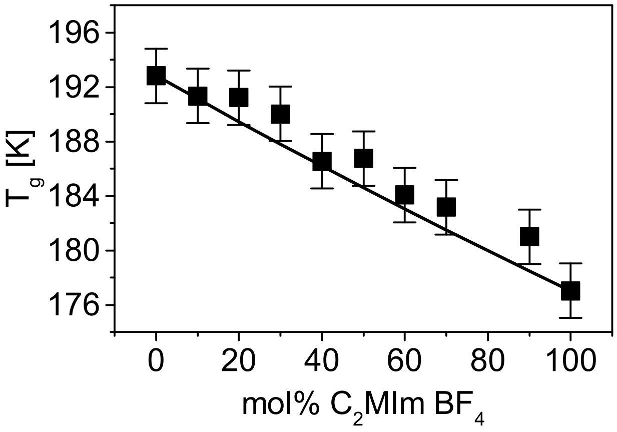


FIG. S2. Calorimetric glass transition temperatures corresponding to the peak maximum of the derivative of heat flow on cooling, see Figure S1. The solid line is the Fox equation.[9]

## DYNAMIC-MECHANICAL AND DIELECTRIC SPECTROSCOPY

The real and imaginary parts of the complex dynamic shear modulus, $G^* = G' + iG''$, are presented in Figure S3(a) for neat $C_8$MIm $BF_4$ and the 30, 50, and 70mol% $C_2$MIm $BF_4$ mixtures. All liquids exhibit viscoelastic behavior depending upon the experimental timescale. The transition from a viscous to an elastic response corresponds with an arrest of molecular motion corresponding to the glass transition. The rate of this structural relaxation, $\omega_{\alpha,DMS}$, corresponds to the crossover point of $G'$ and $G''$. The mechanical relaxation of the majority of liquids deviates from the ideal response of a relaxing Maxwell element due to a broad underlying distribution of relaxations around a mean relaxation rate. Certain liquids which are capable of forming meso- or larger scale heterogeneities also exhibit additional mechanical relaxations at timescales considerably longer than the structural relaxation. This slow relaxation is observed as a low frequency shoulder in the real and imaginary parts of the complex dynamic shear modulus, as a step-change in the real part of complex viscosity and as a peak in the imaginary part of complex viscosity, see Figure S3 (a and b).[10–13] This relaxation was previously observed in the dynamic mechanical spectra of neat $C_8$MIm $BF_4$ and tentatively attributed to fluctuations associated with the existence of mesoscale aggregates.[14] The imaginary part of complex viscosity is fit using a combination of two Cole-Davidson modified Maxwell-relaxation models (Equation 1) providing the relaxation rates of the slow, sub-$\alpha$ and structural, $\alpha$-relaxation rates, $\omega_{slow}$=$1/\tau_{slow}$ and $\omega_\alpha$=$1/\tau_\alpha$, as well as the high-frequency plateau moduli of the two relaxations, $G_{slow}$ and $G_\infty$.[37]

$$\eta'' = G'/\omega = \left[Re\left[G_\infty\left(1 - \frac{1}{(1+i\omega\tau_\alpha)^\gamma}\right) + G_{slow}\left(1 - \frac{1}{(1+i\omega\tau_{slow})^\gamma}\right)\right]\right]/\omega \qquad (1)$$

The fit parameters of the Cole-Davidson modified Maxwell relaxation model, Equation 1, are provided in Tables S1 and S2.

TABLE S1. Fit parameters of Equation 1 for the structural, $\alpha$-relaxation.

| IL | $G_\infty$ [GPa] | $\gamma$ |
|---|---|---|
| $C_8$MIm $BF_4$ | 0.8 | 0.1 |
| 30mol% $C_2$MIm $BF_4$ | 1.5 | 0.1 |
| 50mol% $C_2$MIm $BF_4$ | 1.5 | 0.1 |
| 70mol% $C_2$MIm $BF_4$ | 0.9 | 0.1 |

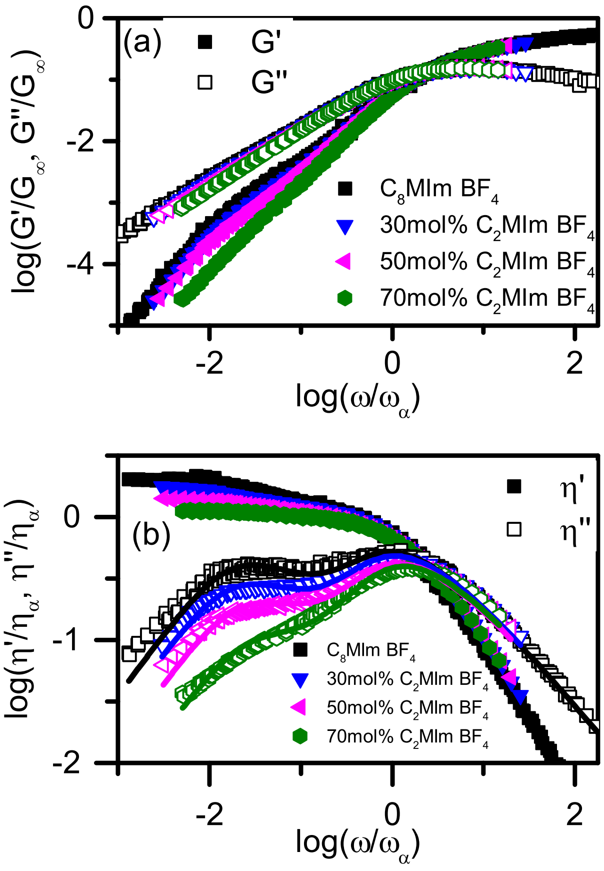


FIG. S3. The real (closed) and imaginary parts (open symbols) of the (a) complex dynamic shear modulus, $G^*(\omega) = G'(\omega) + iG''(\omega)$, and (b) complex viscosity, $\eta^*(\omega) = \eta'(\omega) - i\eta''(\omega)$, as a function of frequency normalized by the structural relaxation rate, $\omega_\alpha$. Lines represent fits by two Cole-Davidson modified Maxwell-models, Equation 1.

TABLE S2. Fit parameters of Equation 1 for slow, sub-$\alpha$-relaxation

| IL | $G_{slow}$[MPa] | $\gamma$ |
|---|---|---|
| $C_8$MIm $BF_4$ | 16 | 0.1 |
| 30mol% $C_2$MIm $BF_4$ | 19 | 0.1 |
| 50mol% $C_2$MIm $BF_4$ | 16 | 0.1 |
| 70mol% $C_2$MIm $BF_4$ | 5.3 | 0.1 |

The relaxation rates obtained as fit parameters of this model, $\omega_{slow,DMS}$ and $\omega_{\alpha,DMS}$, correspond to the rate of the slow and structural relaxations, respectively. While the strength of the slow mechanical relaxation diminishes with increasing $C_2$MIm $BF_4$, the separation

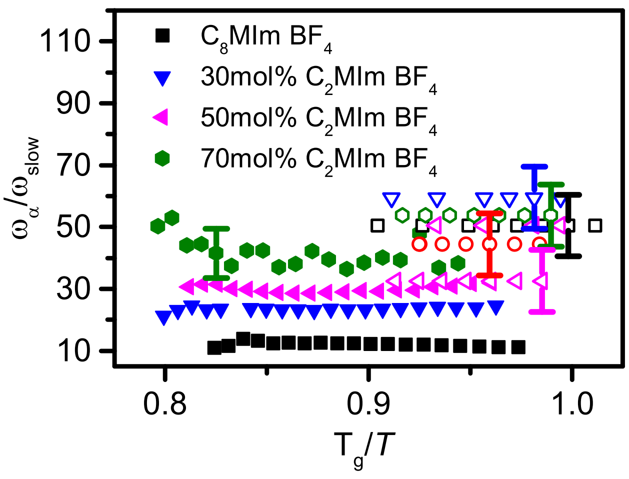


FIG. S4. Relaxation rate ratios *versus* temperature normalized by $T_g$. Closed and open symbols correspond to dielectric and mechanical rates, respectively.

between the two relaxation rates remains relatively constant, Figure S4. This indicates that the volume involved in the mechanical relaxation may not change substantially in the binary mixtures. This is consistent with the relatively slight change in non-polar domain dimensions, as illustrated by the composition dependence of the non-polar correlation distance from x-ray scattering and MD simulations. On the other hand, the weakening of the mechanical relaxation associated with fluctuations of the non-polar domains follows intuitively from the reduction in the overall volume fraction of the non-polar phase and the accompanying reduction in connectivity which occurs upon addition of $C_2$MIm $BF_4$.

The dielectric spectra are presented in Figure S5 for the 50mol% $C_2$MIm $BF_4$ mixture in terms of the real and imaginary parts of the complex dielectric permittivity and conductivity. The spectra are fit with a linear combination of two Havriliak-Negami fitting functions, see Equation 2, where $\tau$ is the model relaxation time, $\Delta\varepsilon$ the dielectric strength, $\varepsilon_\infty$ the high-frequency limiting permittivity, $\sigma_0$ the dc ionic conductivity, $\varepsilon_0$ the vacuum permittivity, and $\beta$ and $\gamma$ are stretching parameters.[15, 16]

$$\varepsilon^*(\omega) = \left[\frac{\Delta\varepsilon_{slow}}{[1+(i\omega\tau_{slow})^\beta]}\right] + \left[\frac{\Delta\varepsilon_\alpha}{[1+(i\omega\tau_\alpha)^\beta]^\gamma}\right] + \frac{\sigma_0}{i\omega\varepsilon_0} + \varepsilon_\infty \tag{2}$$

The low-frequency limiting static dielectric permittivities ($\varepsilon_s = \Delta\varepsilon_{slow} + \Delta\varepsilon_\alpha + \varepsilon_\infty$), the dielectric strengths, and the high-frequency dielectric permittivities are shown in Figure S6(a-d). The dc ionic conductivities are presented Figure S7 alongside the zero-shear viscosities obtained by dynamic-mechanical spectroscopy. The relaxation rates are shown in

Figure S8. The faster relaxation rates measured by dynamic mechanical and broadband dielectric spectroscopy coincide for all measured compositions and scale by the calorimetric glass transition temperature, $T_g$. These relaxations are therefore attributed to the structural relaxation. The slow dielectric relaxation gradually reduces in rate relative to the structural relaxation as the concentration of $C_2$MIm $BF_4$ is increased. The stretching parameters are provided in Figure S9.

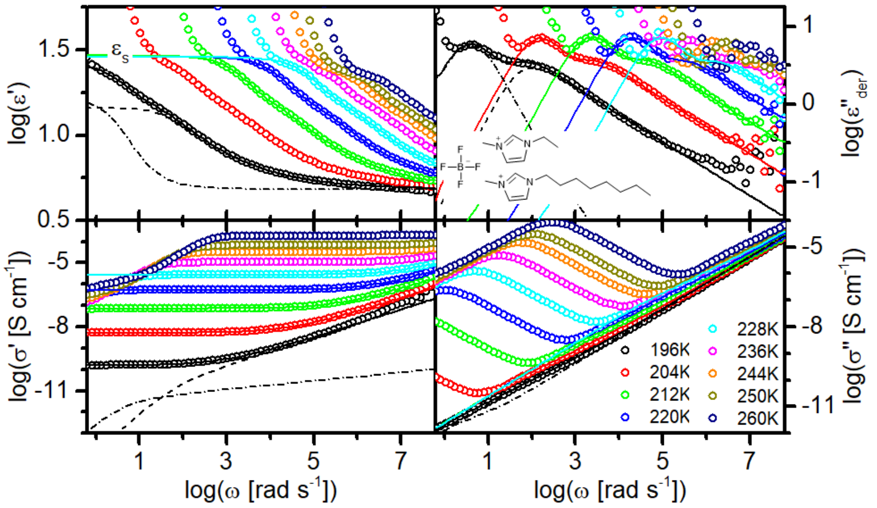


FIG. S5. Real part of complex dielectric function, $\varepsilon'$, the derivative representation of imaginary part of the dielectric function, $\varepsilon''_{der} = (-\frac{\pi}{2})\frac{\partial \varepsilon'}{\partial ln(f)}$, and the real and imaginary parts of complex conductivity, $\sigma^* = \sigma' + i\sigma''$, as functions of frequency and temperature for the 50mol% $C_2$MIm $BF_4$ + $C_8$MIm $BF_4$ mixture. Solid lines represent fits by Equation 2.

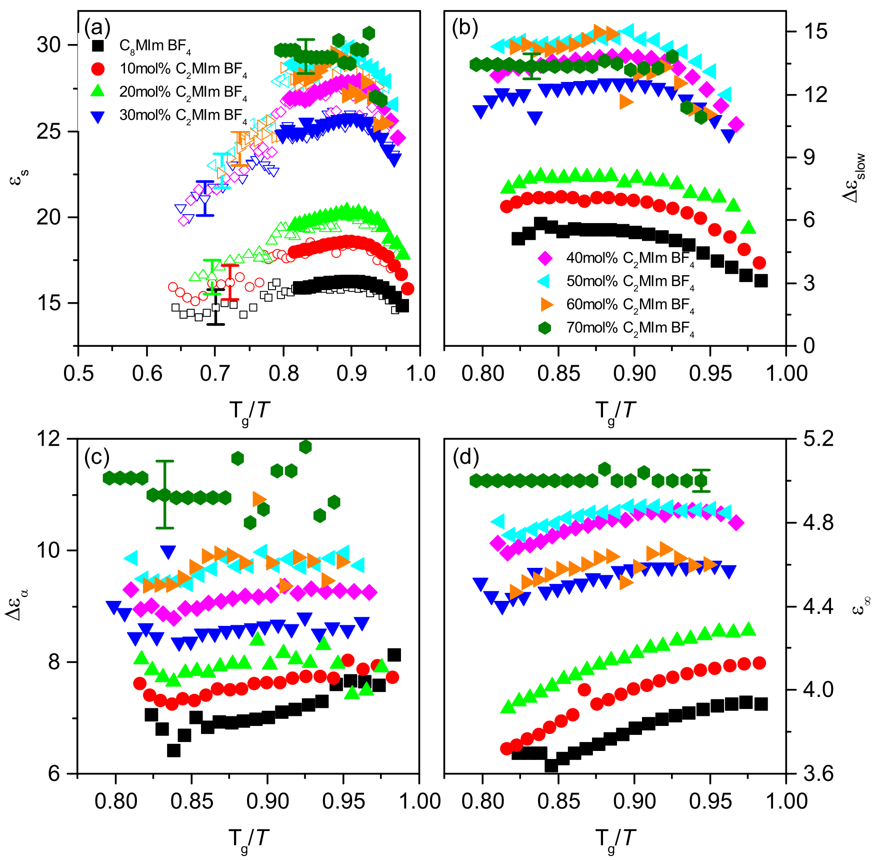


FIG. S6. (a) Static dielectric permittivity, (b) dielectric strength of the slow, sub-$\alpha$ relaxation, (c) dielectric strength of the $\alpha$-relaxation, and (d) the high-frequency limit of the real part of dielectric permittivity for all concentrations *versus* temperature normalized by the calorimetric glass transition temperature. The solid symbols are values from fits by Equation 1. Open symbols are screen-read values of $\varepsilon_s$.

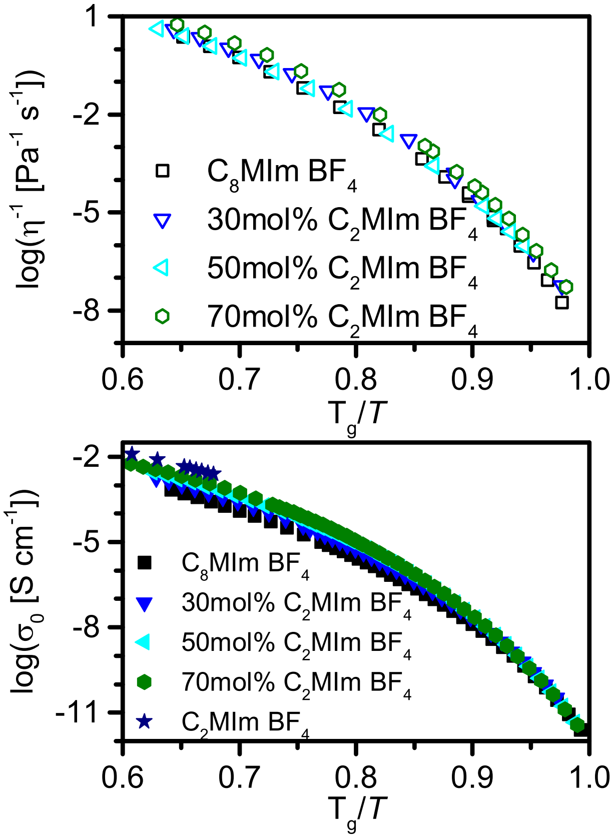


FIG. S7. (a) Fluidity, $\eta^{-1}$, *versus* temperature normalized by $T_g$. (b) DC ionic conductivities, $\sigma_0$, *versus* temperature normalized by $T_g$.

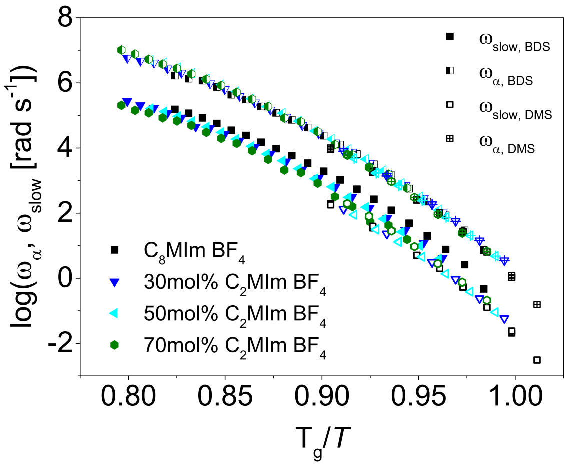


FIG. S8. Relaxation rates of the structural, $\alpha$-relaxation, $\omega_\alpha$, and the slow, sub-$\alpha$ relaxation, $\omega_{slow}$, as obtained by dielectric and mechanical spectroscopy *versus* temperature normalized by the calorimetric glass transition temperature, $T_g$.

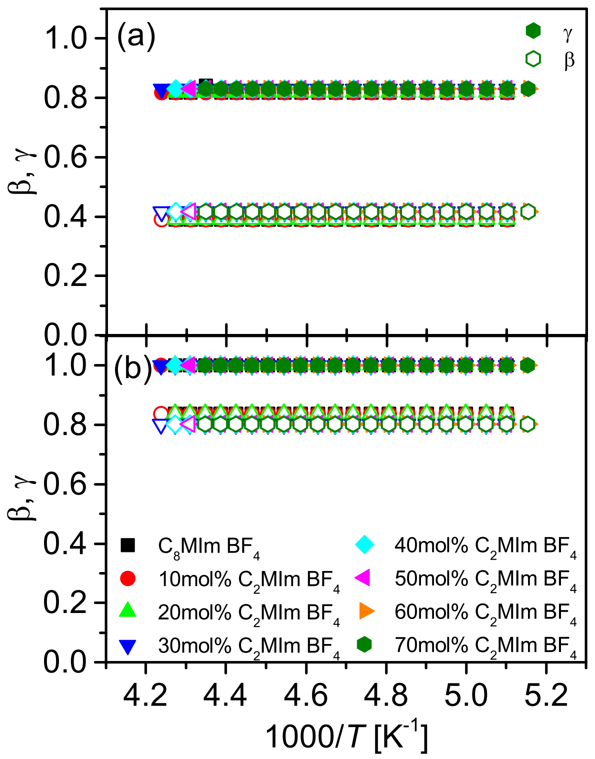


FIG. S9. Shape parameters, $\beta$ (open symbols)and $\gamma$ (closed symbols, of Cole-Cole and Havriliak-Negami equations used to fit the dielectric spectra. (a) Shape parameters of the structural, $\alpha$ relaxation. (b) Shape parameters of the slow, sub-$\alpha$ relaxation.

A comparison of relaxation rates obtained by Equation 2 and those obtained by the random barrier model is shown in Figure S10 for 50mol% $C_2$MIm $BF_4$. In the random barrier model, the ions are taken to be hopping in a randomly varying energy landscape. The onset of dc ionic conductivity, $\sigma_0$, corresponds to the time, $\tau_{RBM}$, it takes for ions to overcome the largest energy barrier to form a percolated conducting path. Solved within the continuous time random walk approximation an analytical expression for the complex dielectric function is obtained which contains only two parameters, the dc ionic conductivity and the ion hopping rate, $\sigma_0$ and $\omega_{RBM}$, respectively.[17] This model describes the frequency dependence of the real part of complex conductivity for ion conducting liquids and glasses quite well. The structural, $\alpha$-relaxation rates, $\omega_\alpha$ coincide with the ion hopping rates, $\omega_{RBM}$.

The dielectric spectra of the 80mol% $C_2$MIm $BF_4$ mixture are provided in Figure S11 in terms of the derivative representation $\Delta\varepsilon_{der}$. Above 70mol% $C_2$MIm $BF_4$, the slow dielectric relaxation is not observed as shown in Figure S11. This is attributed to a disruption of the

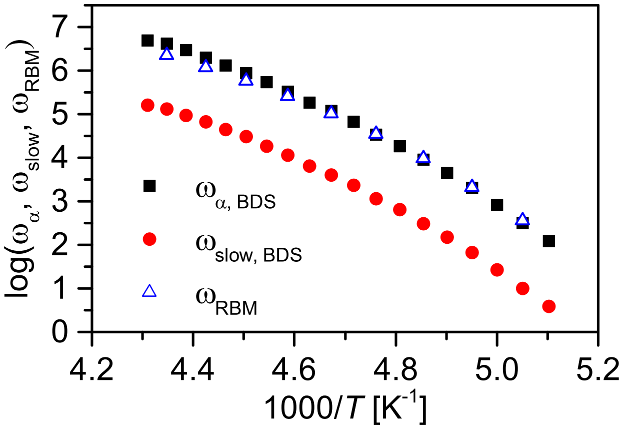


FIG. S10. Dielectric relaxation rates of 50mol% $C_2$MIm $BF_4$ obtained by Equation 2 and the random barrier model, $\omega_{RBM}$.

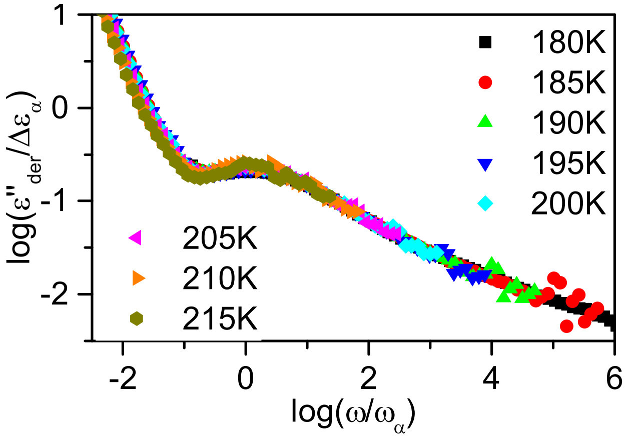


FIG. S11. The derivative representation of the imaginary part of the complex dielectric function, $\varepsilon''_{der} = (-\frac{\pi}{2})\frac{\partial \varepsilon'}{\partial ln(f)}$, for 80mol% $C_2$MIm $BF_4$. The structural, $\alpha$-relaxation is more fully resolved than at any lower $C_2$MIm $BF_4$ concentration and there is no evidence of a slower sub-$\alpha$ relaxation.

mesoscale aggregates above a critical concentration of $C_2$MIm $BF_4$.

The symmetric Looyenga effective medium approximation is give in Equations 3 and 4:

$$\varepsilon_s = \frac{1}{\sigma_0}\left[\sigma_s\varepsilon_1 - \left(\frac{\sigma_2}{\sigma_s}\right)^{-2n}\phi\big(\sigma_2\varepsilon_1 - \sigma_1\varepsilon_2\big)\right] \tag{3}$$

$$\sigma_0^{1-2n} = \sigma_1^{1-2n} + \phi\big(\sigma_2^{1-2n} - \sigma_1^{1-2n}\big) \tag{4}$$

where subscript 1 signifies the polar phase, subscript 2 the non-polar phase, $\sigma_0$ the measured dc ionic conductivity of the mixture taken at T=1.5T$_g$, $\sigma_1 = 3.4 \times 10^{-3}\,\mathrm{S\,cm^{-1}}$ is the dc ionic conductivity of pure $C_2$MIm $BF_4$ at T=1.5T$_g$, $\varepsilon_1 = \Delta\varepsilon_\alpha + \varepsilon_\infty$ taken at T=1.1T$_g$ in Figure

S6, $\sigma_2$=$4 \times 10^{-6}\,\mathrm{S\,cm^{-1}}$ $\varepsilon_2 = 1.8$ the static dielectric permittivity of hexane as a reasonable model of the non-polar phase.[18] The remaining variables, $\phi$, and n, corresponding to the volume fraction, and shape of the insulating phase, were used as free fit parameters until the two equations gave converging values of $\varepsilon_s$ and $\sigma_0$ approximately equal to the measured quantities, see Figure S12. With increasing $C_2$MIm $BF_4$ concentration, the measured $\varepsilon_s$ is predicted only if n approaches 0.33.

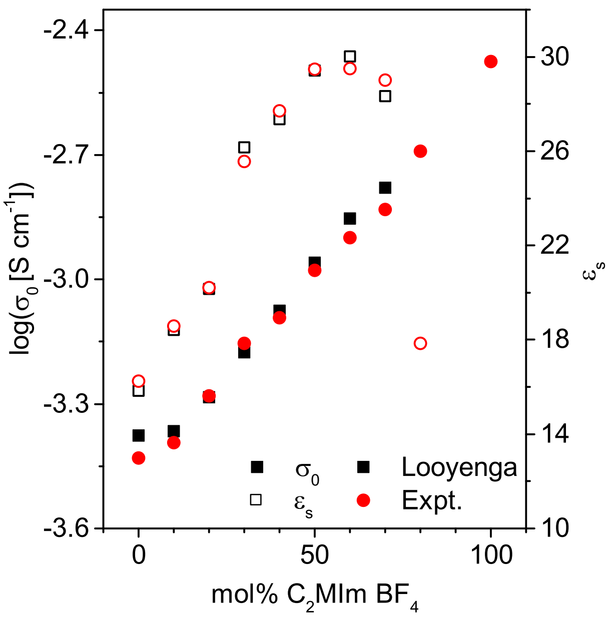


FIG. S12. (a) DC ionic conductivity, $\sigma_0$, at T=1.5T$_g$ (closed squares) and static dielectric permittivity, $\varepsilon_s$, at T=1.1T$_g$ (open squares), as well as estimates of $\sigma_0$ and $\varepsilon_s$ from the Looyenga EMA (closed and open circles) *versus* $C_2$MIm $BF_4$ concentration.

## MOLECULAR DYNAMICS RESULTS

### Force Field

A classical all-atom force field model developed by Canongia Lopes-Pádua [3, 4] (CL&P) that have the following functional form for computing intramolecular and intermolecular

interactions:

$$E_{tot} = \sum_{ij}^{\text{bonds}} \frac{k_{r,ij}}{2}(r_{ij} - r_{0,ij})^2 + \sum_{ijk}^{\text{angles}} \frac{k_{\theta,ijk}}{2}(\theta_{ijk} - \theta_{0,ijk})^2$$
$$+ \sum_{ijkl}^{\text{torsions}} \sum_{m=1}^{4} \frac{k_{m,ijkl}}{2}[1 + (-1)^{m+1}\cos(m\phi_{ijkl})] +$$
$$+ \sum_{ij}^{\text{nonbonded}} \left\{ 4\epsilon_{ij} \left[ \left(\frac{\sigma_{ij}}{r_{ij}}\right)^{12} - \left(\frac{\sigma_{ij}}{r_{ij}}\right)^{6} \right] + \left(\frac{q_i q_j}{r_{ij}}\right) \right\} \tag{5}$$

where $k_{r,ij}$, $k_{\theta,ijk}$, $k_{m,ijkl}$ represent the force constants for bond stretching, angle bending, torsion (both proper and improper), respectively, $\epsilon$ and $\sigma$ indicate the Lennard-Jones 12-6 energy and size parameters, and $q$ denotes partial charges; is a well parameterized and transferable force field that encompasses homologous series of imidazolium-based cations with arbitrary chain lengths and multiple anions. Thus, 1-n-octyl-3-methylimidazolium $C_8MIm^+$ and 1-ethyl-3-methylimidazolium $C_2MIm^+$ cations and tetraborofluorate $BF_4{}^-$ anion were modeled using CL&P force field. The Lennard-Jones unlike interactions were computed by the geometric-mean combining rule for both the parameters. The intramolecular 1-4 non-bonded interactions were reduced by a factor of 2, however, such interactions were excluded for the atoms connected by bonds and angles. The total charge on the cation and anion is $\pm$ 1.

**Structure Factors**

The structure factors, $S(q)$, were calculated using eq. 6;

$$S_{ij}(q) = \frac{\rho_o x_i x_j f_i(q) f_j(q) \int_0^R 4\pi r^2 \left[g_{ij}(r) - 1\right] \frac{\sin(qr)}{qr} \left(\frac{\sin(\frac{\pi r}{R})}{\frac{\pi r}{R}}\right) dr}{\left[\sum_i x_i f_i(q)\right]^2} \tag{6}$$

where $S_{ij}(q)$ is the partial structure factor obtained from the Fourier transform of the radial distribution function, $g_{ij}(r)$, between the atoms of type $i$ and $j$, $\rho_o$ is the average atomic number density, $x_i$ is the atomic fraction of $i$, $q$ is the scattering vector, and $f_i(q)$ is the X-ray atomic form factor for the atom type $i$ taken from the International Tables for Crystallography.[19] $R$ represents the cutoff distance defined for calculating $g_{ij}$(r). A Lorch type window function, $\left(\frac{\sin(\frac{\pi r}{R})}{\frac{\pi r}{R}}\right)$, is also used to attenuate the effect of using finite cutoff

in calculating the radial distribution function between the atoms types $i$ and $j$.[20] The structure factors were computed using TRAVIS[6, 7] after including the Lorch type function in the source code. Half of the simulation box length, $R$, was used as the cutoff distance for these calculations.

### Qualitative Snapshots

Instantaneous snapshots of the equilibrated ionic liquids and binary ionic liquid mixtures are presented in Figure S13. The color scheme is illustrated in the inset.

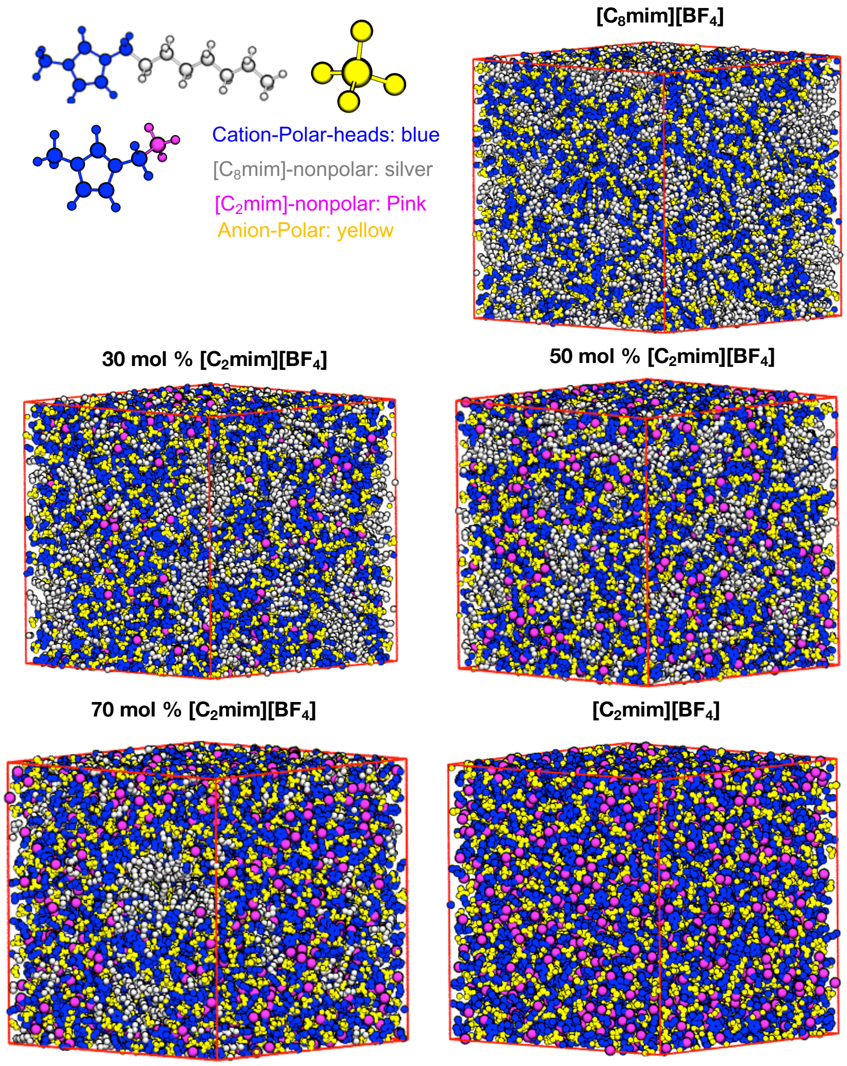


FIG. S13. Instantaneous snapshot of the equilibrated system for $C_8$MIm $BF_4$, $C_2$MIm $BF_4$ and the 30, 50, and 70mol% $C_2$MIM $BF_4$ binary mixtures. The snapshots are color-coded to reflect the polar and nonpolar components on both cation and anion. (Cation-polars: blue, Anion: yellow, $C_8$MIm-nonpolar: silver, and $C_2$MIm-nonpolar: pink).

---


[1] E. Lindahl, B. Hess, and D. van der Spoel, GROMACS 3.0: A Package for Molecular Simulation and Trajectory Analysis, Molecular modeling annual **7**, 306 (2001).

[2] M. J. Abraham, D. van der Spoel, E. Lindahl, B. Hess, , and the GROMACS development team, GROMACS User Manual Version 5.0.4, www.gromacs.org, Journal of Molecular Modeling

(2014).

[3] J. N. Canongia Lopesand A. A. H. Pádua, Molecular force field for ionic liquids iii: Imidazolium, pyridinium, and phosphonium cations; chloride, bromide, and dicyanamide anions, The Journal of Physical Chemistry B **110**, 19586 (2006).

[4] J. N. Canongia Lopes, A. A. H. Pádua, and K. Shimizu, Molecular force field for ionic liquids iv: Trialkylimidazolium and alkoxycarbonyl-imidazolium cations; alkylsulfonate and alkylsulfate anions, The Journal of Physical Chemistry B **112**, 5039 (2008).

[5] L. Martínez, R. Andrade, E. G. Birgin, and J. M. Martínez, PACKMOL: A Package for Building Initial Configurations for Molecular Dynamics Simulations, Journal of Computational Chemistry **30**, 2157 (2009).

[6] M. Brehmand B. Kirchner, TRAVIS - A Free Analyzer and Visualizer for Monte Carlo and Molecular Dynamics Trajectories, Journal of Chemical Information and Modeling **51**, 2007 (2011).

[7] M. Brehm, H. Weber, M. Thomas, O. Hollóczki, and B. Kirchner, Domain Analysis in Nanostructured Liquids: A Post-Molecular Dynamics Study at the Example of Ionic Liquids, ChemPhysChem **16**, 3271 (2015).

[8] W. Humphrey, A. Dalke, and K. Schulten, VMD: Visual molecular dynamics, Journal of Molecular Graphics **14**, 33 (1996).

[9] P. C. Hiemenzand T. P. Lodge, *Polymer Chemistry*, 2nd ed. (CRC Press, New York, 2007).

[10] C. Gainaru, M. Wikarek, S. Pawlus, M. Paluch, R. Figuli, M. Wilhelm, T. Hecksher, B. Jakobsen, J. C. Dyre, and R. Böhmer, Oscillatory Shear and High-pressure Dielectric Study of 5-methyl-3-heptanol, Colloid and Polymer Science **292**, 1913 (2014).

[11] T. Hecksherand B. Jakobsen, Communication: Supramolecular Structures in Monohydroxy Alcohols: Insights from Shear-mechanical Studies of a Systematic Series of Octanol Structural Isomers, The Journal of Chemical Physics **141**, 101104 (2014).

[12] T. Hecksher, Communication: Linking the Dielectric Debye Process in Mono-alcohols to Density Fluctuations, The Journal of Chemical Physics **144**, 4 (2016).

[13] S. Arrese-Igor, A. Alegría, and J. Colmenero, Multimodal Character of Shear Viscosity Response in Hydrogen Bonded Liquids, Physical Chemistry Chemical Physics 10.1039/C8CP04183K (2018).

[14] T. Cosby, Z. Vicars, Y. Wang, and J. Sangoro, Dynamic-Mechanical and Dielectric Evidence of Long-Lived Mesoscale Organization in Ionic Liquids, The Journal of Physical Chemistry Letters **8**, 3544 (2017).

[15] S. Havriliakand S. Negami, A Complex Plane Analysis of $\alpha$-dispersions in Some Polymer Systems, Journal of Polymer Science Part C: Polymer Symposia **14**, 99 (1966).

[16] F. Kremerand A. Schönhals, *Broadband Dielectric Spectroscopy* (Springer, Berlin, 2003).

[17] J. C. Dyre, The Random Free˜energy Barrier Model for AC Conduction in Disordered Solids, Journal Applied Physics **64**, 2456 (1988).

[18] F. I. Mopsik, Dielectric Constant of N-Hexane as a Function of Temperature, Pressure, and Density, Journal of Research of the National Bureau of Standards -A. Physics and Chemistry **71** (1967).

[19] P. J. Brown, A. G. Fox, E. N. Maslen, M. A. O'Keefe, and T. M. Willis, International Tables for Crystallography, Prince, E., Ed. International Union of Crystallography: Dordrecht,The Netherlands **C**, 554 (2004).

[20] E. Lorch, Neutron Diffraction by Germania, Silica and Radiation-Damaged Silica Glasses, Journal of Physics C: Solid State Physics **2**, 229 (1969).
